# Supplementary material for: Coherence of a charge stabilised tin-vacancy spin in diamond
Source: arXiv:2110.05451 source file (2022-05-27)
Supplement: Supplementary file 1 [file SupplementaryInformation.pdf]

# Supplementary Information

March 18, 2022

## Supplementary note 1: Single Emitter Characterisation

### Spectra and ground state splittings

In this section the spectra of the investigated $SnV^-$centres are displayed in Supplementary Figure 1 and evaluated with respect to their ground state splitting as an indicator of strain. All spectra are measured under off resonant excitation. The ground state splittings are 819 GHz, 817 GHz and 820 GHz for emitter 1,2 and 3 respectively. This indicates that all of them are experiencing almost no strain, which is a result of the HPHT annealing.

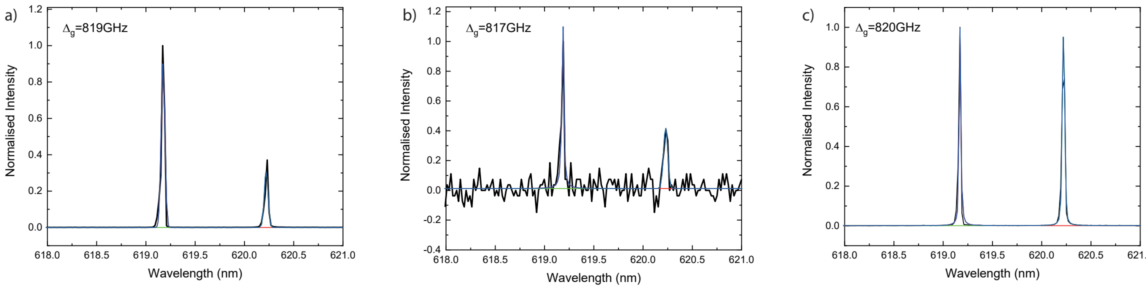


Supplementary Figure 1: **Spectra of the investigated $SnV^-$centres:** Spectra of **a)** emitter 1, **b)** emitter 2 and **c)** emitter 3 exhibiting the spectral finger print of the $SnV^-$centre with a ground state splitting of **a)** 819 GHz, **b)** 817 GHz and **c)** 820 GHz respectively. The ground state splittings of all three emitters being close to the ideal value of around 820 GHz is a measure of vanishing strain induced by the diamond lattice.

### Autocorrelation measurements

We measure the autocorrelation function $g^2(\tau)$ of the photons emitted into the phononic sideband of the investigated emitters under continuous resonant excitation on the C-transition and no magnetic field applied. The results for emitter 1 and 3 are shown in Supplementary Figure 2. We measure raw data values of $g^2(0) = 0.07$ for emitter 1 and $g^2(0) = 0.13$ for emitter 3 without any background or APD dark counts correction. We furthermore emphasize that every investigated emitter in this sample exhibits bunching, some times on several hundreds of microseconds timescales, which is consistent with the charge processes discussed in the main text. This is depicted in Supplementary Figure 2c) and d) for the two emitters. The bunching decays mono-exponentially with a time constant of $\tau_{\text{bunching}} = 90\,\mu s$ ($\tau_{\text{bunching}} = 79\,\mu s$) for emitter 1 (emitter 3) at a blue laser power of about 100 µW (70 µW ). For emitter 2 no autocorrelation measurement was taken, but the single emitter character was confirmed via PLE scans exhibiting only a single resonance line and furthermore CPT measurements exhibiting only a single dip even for the lowest power measurement in the main text with a power broadened dip width of about 160 kHz (64 kHz resulting from the spin coherence time, the rest from residual power broadening).

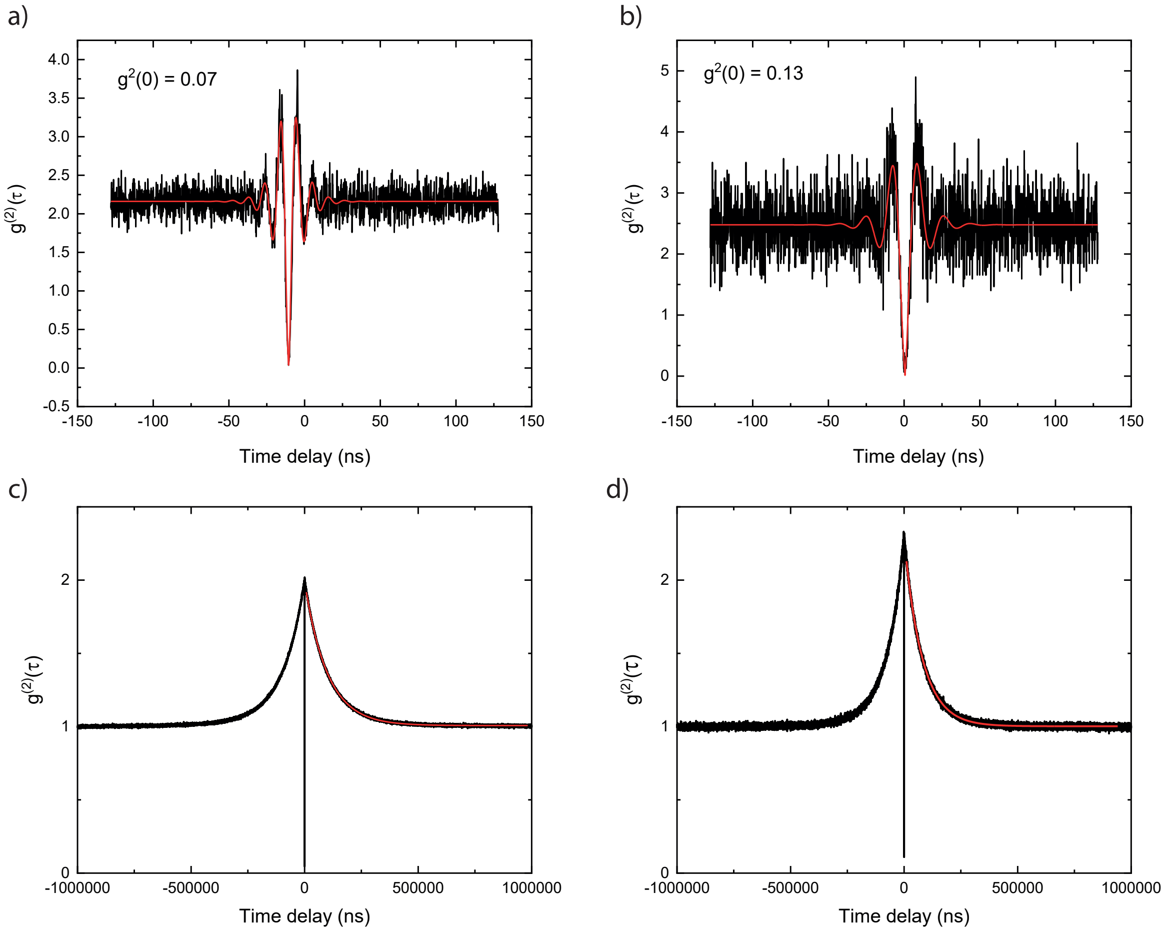


Supplementary Figure 2: **Autocorrelation measurements of single $SnV^-$centres: a)** Autocorrelation measurement of emitter 1 under continuous resonant excitation on the C-transition and collection of photons emitted into the phononic sideband, exhibiting a raw data value $g^2(0) = 0.07$ pinpointing the single photon emission character of the emitter. **b)** Same measurement for emitter 3, exhibiting a raw data value $g^2(0) = 0.13$ also indicating single photon emission. Long range correlation of the emitted fluorescence exhibits the typical bunching decay resulting from the charge termination and subsequent charge repump discussed in the main paper. The time constant of the decay is **c)** $\tau_{\text{bunching}} = 90\,\mu s$ and **d)** $\tau_{\text{bunching}} = 79\,\mu s$.

# Supplementary note 2: Fluorescence enhancement measurement in sample NI58

For the fluorescence enhancement measurement in Figure 1b) of the main text, we here present the count rate data values without normalisation. Due to the different scales, the enhancement and excitation probability curves are depicted in two separate graphs. In Supplementary Figure 3a), we show the count rate emitted by the ensemble upon application of the resonant as well as the second colour light field as function of the second laser wavelength. The red star indicates the count rate emitted under application of the resonant excitation light field only. In Supplementary Figure 3b) the count rate upon direct excitation of the ensemble with the second light field only is depicted.

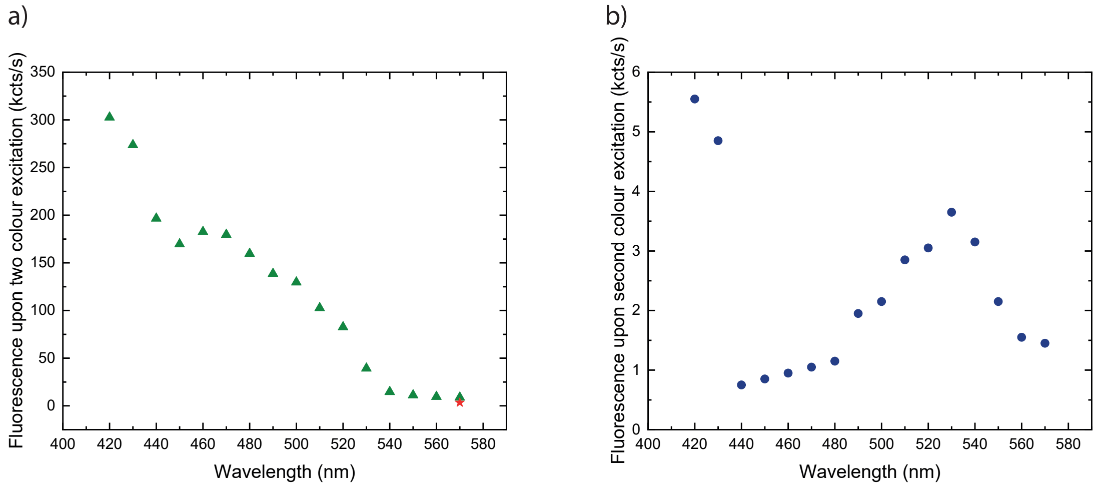


Supplementary Figure 3: **Count rate data of the fluorescence enhancement measurement:** Depicted is the count rate data corresponding to Figure 1b) of the main text. In **a)** the count rate upon excitation with resonant and charge stabilisation light fields being applied is depicted. The red star indicates the count rate emitted with only the resonant excitation light field being applied. **b)** Shown is the count rate emitted for only the charge stabilisation light field exciting the ensemble.

# Supplementary note 3: Additional HPHT sample

In this section we briefly confirm the charge stabilisation for a second HPHT sample (BOJO_001). We repeat the fluorescence enhancement measurement presented in the main text and find the result in very good agreement, see Supplementary Figure 4. Also in this measurement we find indication of an even higher lying excited state for excitation energies larger than 2.8 eV, although it is less pronounced than in the measurement presented in the main paper. Both measurements are conducted in dense implantation regions (about $10^{12}\,\frac{\mathrm{Ions}}{\mathrm{cm}^2}$), where a lot of lattice damage is induced. Sample BOJO_001 is HPHT annealed for 2 h compared to 20 min for sample NI58 thus we expect less strain for the former. A likely candidate for the resonance at 2.8 eV is a transition from a deep $a_{1g}$ state in the valence band (discussed for the $SiV^-$ centre in [1] (Figure 2), but universal to all G4V centres) to the $e_g$ level of the $SnV^-$ centre. As this transition is parity forbidden, it becomes more probable with increasing strain. As we cannot fully access the transition with our current laser systems, a proper characterisation and identification remains subject to future investigations. Also for this sample we find that application of 445 nm laser radiation reliably initialises the charge state of every emitter under investigation. For charge stabilised emitters, we measure pure single photon emission ($g^2(0) = 0.06$ without any background substraction, Supplementary Figure 5a)) under resonant excitation and find the resonance of the C-transition to be long-term stable (Supplementary Figure 5b)). The long-term PLE measurement is conducted in a power regime of the resonant excitation laser where electron capture occurs in every scan and the stabilisation laser is continuously applied. These measurements show that the concepts presented in the main paper can be universally applied to ion implanted HPHT samples.

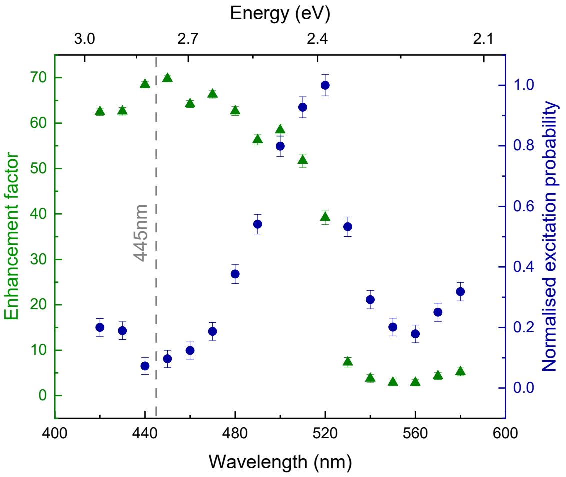


Supplementary Figure 4: **Fluorescence enhancement measurement:** Repetition of the measurement on the enhancement of fluorescence factor of an ensemble of $SnV^-$centres in the second HPHT sample. The ensemble is excited resonantly on the C-transition and under addition of a second laser with tunable wavelength. The enhancement factor is defined as stated in the main text. For comparison, the normalised excitation probability measured via excitation by the second laser only is plotted. The excitation probability peaks at ˜2.4 eV due to excitation to a higher excited state of the SnV [2] and also in the second sample the indication of an even higher lying excited state is seen at photon energies larger 2.8 eV most likely resulting from a deeper lying electron state in the valence band [3]. y-errors (s.d.): Poisson distributed count rate errors.

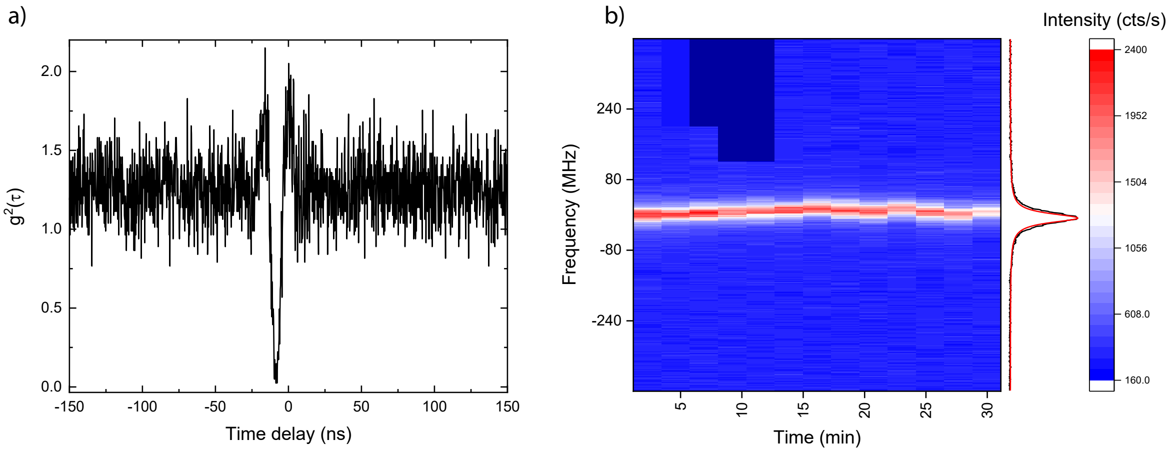


Supplementary Figure 5: **Autocorrelation and long-term PLE: a)** Autocorrelation of a single emitter in the second HPHT sample under resonant excitation exhibiting almost perfect single photon emission indicated by $g^2(0) = 0.06$ before any background substraction. **b)** Long-term PLE measurement of the C-transition in a power regime where electron capture occurs in every scan and the charge stabilisation laser is continuously applied. On the right, the integrated spectrum over all scans (black) with a width of 31(2) MHz is compared with the Fourier limited spectrum (red, 25 MHz)

## Supplementary note 4: SiV ensemble

We repeat the wavelength dependent fluorescence enhancement measurement, that was presented in the main text, for an ensemble of $SiV^-$ centres. The excitation is achieved by continuously exciting the ensemble on the C-transition with a continuous wave TiSa laser. The second light field is provided by the supercontinuum laser and kept at constant power throughout the measurement. As it is obvious from Supplementary Figure 6, we again see a strong increase in the enhancement of the fluorescence for energies of the second photon exceeding 2.4 eV. Due to this measurement being performed in a different optical setup, we were limited by the employed optics for photon energies above 2.8 eV. The absolute value of the enhancement is lower than in the measurement on the SnV ensemble in the main text, which results from a higher resonant laser power used. This higher power is sufficient to drive the (0/-) charge transition of the divacancy via a two photon process. For lower resonant laser powers we observed enhancement factors larger than 10. We would also like to comment on the fact, that $SiV^-$ fluorescence is usually not completely terminated under resonant excitation. A possible reason for this is that the lower energy state of the $SiV^{2-}$ centre, in contrary to the $SnV^{2-}$, lies within the valence band and therefore a continuous capture and release of electrons is possible.

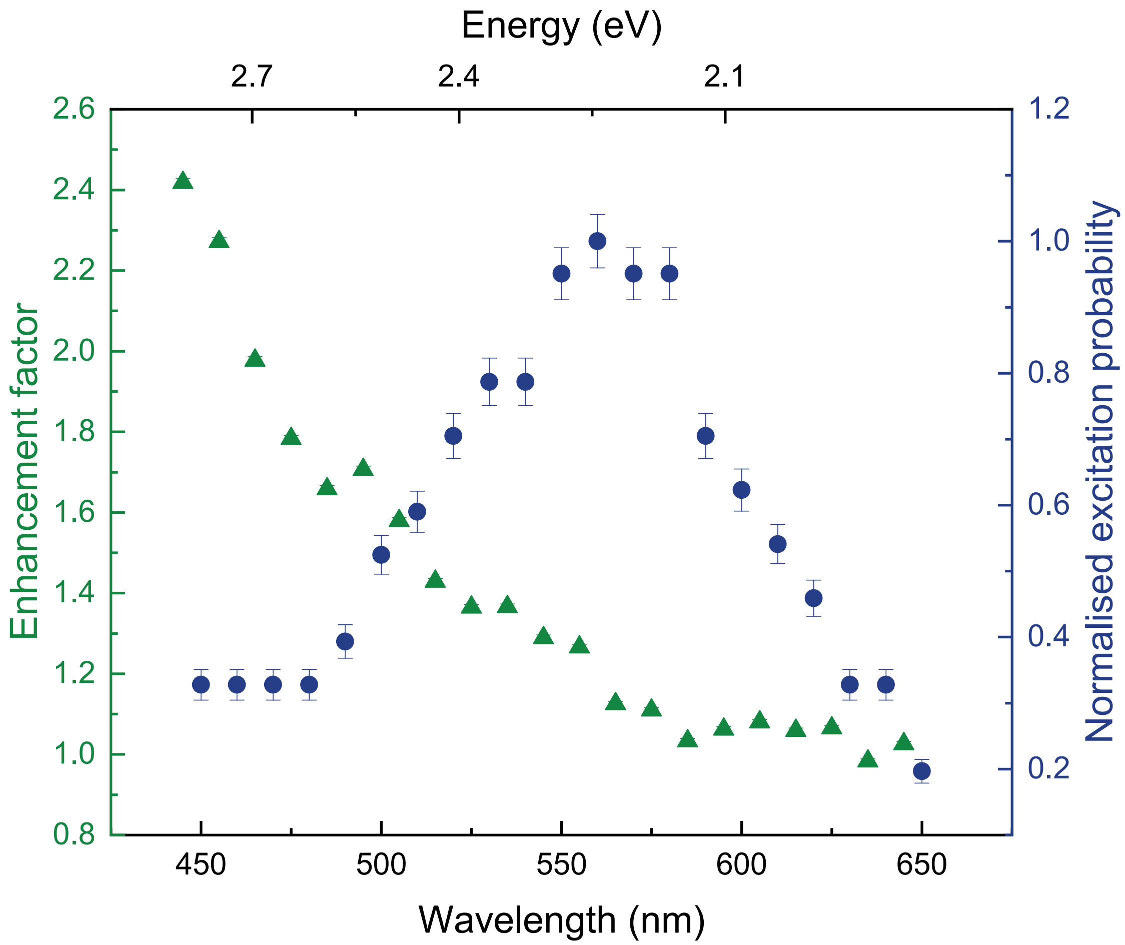


Supplementary Figure 6: **Enhancement of fluorescence for $SiV^-$ centres:** Measurement of the enhancement of fluorescence factor of an ensemble of $SiV^-$centres, excited resonantly on the C-transition under addition of a second laser with tunable wavelength. As for the case of the $SnV^-$centres, a steep rise for photon energies of the second light field exceeding 2.4 eV is visible. y-errors (s.d.): Poisson distributed count rate errors.

# Supplementary note 5: Spin lifetime

We measure the spin lifetime by applying a pulse sequence constisting of two 300 $\mu$s (200 $\mu$s) long pump pulses for emitter 1 and 3 (2) resonant with the SC A1 transition separated by a variable pulse delay. The first pulse initialises more than 97 % of the population in the state $|2\uparrow\rangle$ and the second pulse reads out the amount of population decaying back to state $|1\rangle$ during the delay time. From the ratio of the pulse heights from read to initialisation pulse for variable delays, we can extract the spin lifetime $T_1$, which is 21(2) ms, 22(5) ms and 15(1) ms for emitter 1,2 and 3 at a magnetic field of $B$=200 mT ($B$=80 mT for emitter 3) and Temperature $T$=1.7 K (see Supplementary Figure 7). The charge stabilisation during the measurements is either provided by an inital 10 ms long blue pulse at the beginning of each pulse sequence (emitter 1) or by continuous illumination with 445 nm laser light (emitter 2 and 3).

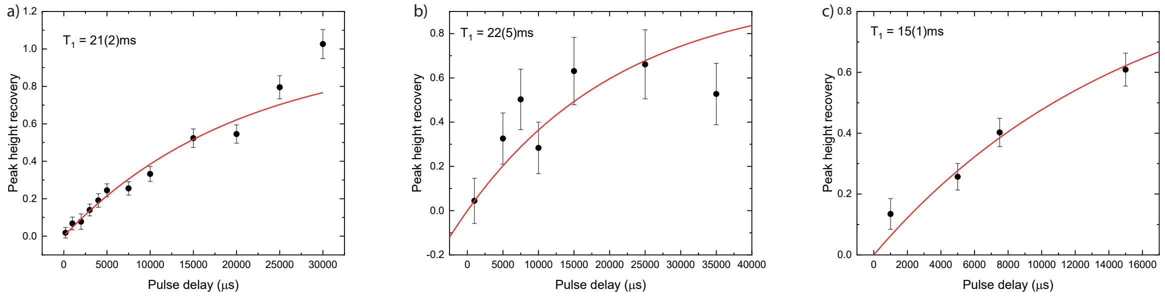


Supplementary Figure 7: **Spin lifetime measurement:** Measurement of the spin lifetime at a magnetic field of $B$=200 mT and temperature of 1.7 K yielding **a)** $T_1$=21(2) ms for emitter 1, **b)** $T_1$=22(5) ms for emitter 2 and **c)** $T_1$=15(1) ms for emitter 3. y-errors (s.d.): Poisson distributed count rate errors.

# Supplementary note 6: Charge processes of additional emitters and long-term PLE

The results for the electron capture mechanism and the charge initialisation that are discussed in the main text are reproduced on a second emitter. In Supplementary Figure 8 the electron capture rate is measured with a pulse sequence of 500 $\mu$s blue laser on, 100 $\mu$s waiting time and a subsequent 6 s long red laser pulse being resonant with the C-transition. The experiment was repeated for each red laser power until about 230 fluorescence responses were recorded. The same linear dependency of the electron capture rate on the excitation power and a power dependent electron capture rate on the same order of magnitude are observed as for emitter 1 (see main text). Furthermore, we also measure the initialisation efficiency with a slightly altered pulse sequence using a fixed red power and varying the pulse length of the blue laser. The power of the blue laser corresponds to 90 µW cw power. We evaluate the measurement in the same way as in the main text, count the number of fluorescence responses and divide them by the total number of initialisation pulses sent to the emitter. As displayed in Supplementary Figure 8 b), we reach an initialisation efficiency derived from the exponential growth fit of 97(2) % with a time constant $\tau_{\mathrm{CI}}$ =657(43) µs. These results are in good agreement with the findings on emitter 1 in the main text. The method of efficient charge initialisation by illumination with blue light did work on several tens of emitters that were investigated in this sample and furthermore also in ensemble regions. In very few cases we still observed blinking of the fluorescence which we attribute to non-perfect alignment of the blue laser light spot with respect to the emitter.

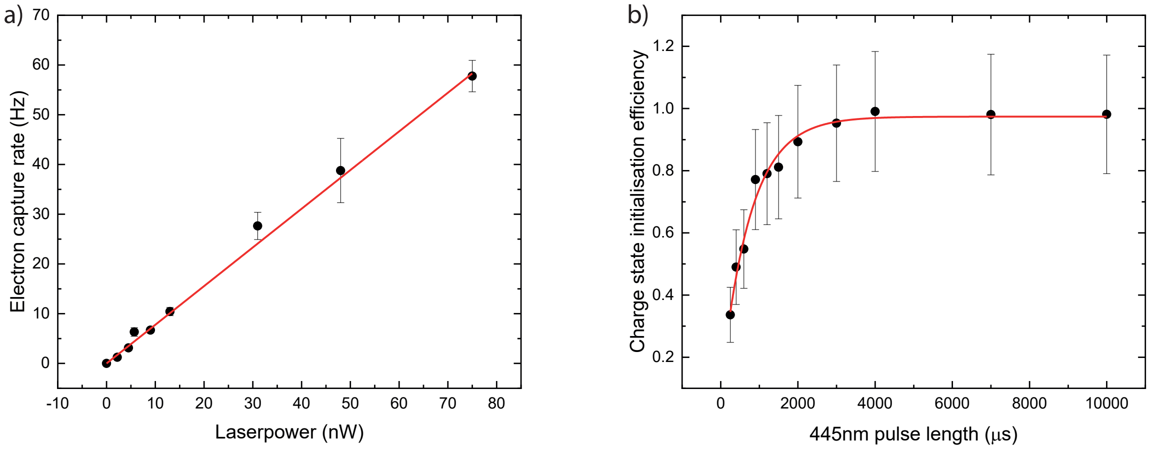


Supplementary Figure 8: **Charge processes of emitter 3: a)** Electron capture rate plotted against the incident laser power. The linear dependency indicates a single photon process. y-errors (s.d.): Fitting errors from exponential fit of charge lifetime histogram. **b)** Charge state initialisation efficiency for varying length of the blue laser pulse (power: 90 μW). The efficiency saturates with a time constant $\tau_{\mathrm{CI}} = 657(43)\,\mu\mathrm{s}$ at 97(2) %, yielding almost perfect charge initialisation. y-errors (s.d.): Poisson distributed count rate errors.

The dependence of the time constant $\tau_{\mathrm{CI}}$ and the corresponding charge initialisation rate $\gamma_{\mathrm{CI}} = \frac{1}{\tau_{\mathrm{CI}}}$ on the blue laser power is evaluated for an additional emitter 4. We measure the charge initialisation rate as before and vary the blue laser power. As expected from the charge cycle model proposed in the main text, the rate increases linearly with laser power corresponding to a single photon process, which is depicted in Supplementary Figure 9. The slope of this increase is extracted from the linear fit to be $190(8)\,\frac{\mathrm{Hz}}{\mu\mathrm{W}}$ and the y intercept set to zero. For each laser power, charge initialisation efficiencies in between 85 %-90 % are reached, thus faster initialisation and high initialisation efficiency are not traded off against each other.

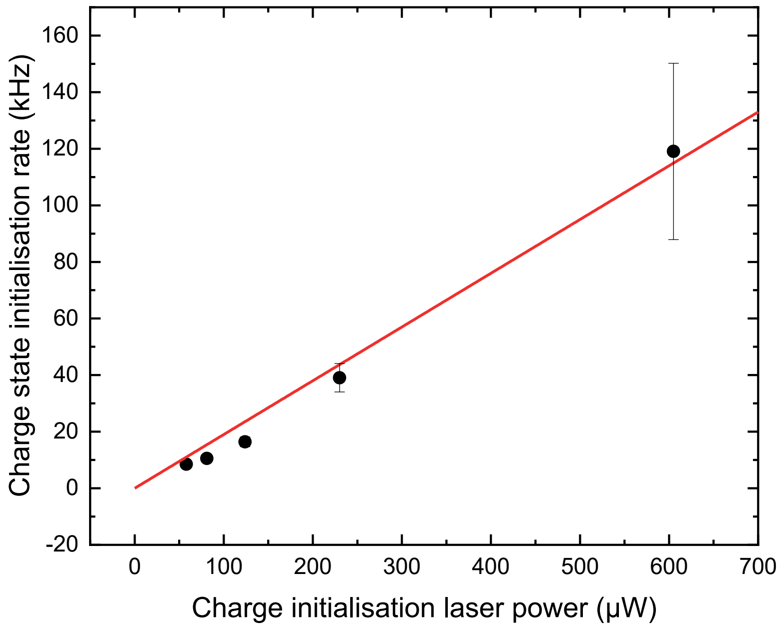


Supplementary Figure 9: **Power dependence of the charge initialisation rate:** We measure the charge initialisation rate for different laser powers of the 445 nm laser. As expected from the model proposed in the main text, the rate increases linearly with a slope of $190(8)\,\frac{\mathrm{Hz}}{\mu\mathrm{W}}$. For each blue power, highly efficient charge initialisation ranging in between 85 %-90 % is reached, thus rapid charge initialisation with high efficiency is feasible. y-errors (s.d.): Fitting errors from exponential fit of charge initialisation curve.

It is interesting to compare the effect of charge stabilisation with 445 nm laser light to the case of utilising the standard 532 nm radiation. In Supplementary Figure 10 PLE scans probing the spectral stability of emitter 4 for the two cases are depicted with a resonant excitation power of 1 nW and the charge stabilisation laser being applied continuously with 10 µW. It is obvious that the 445 nm charge stabilisation provides a clean, bright spectral line. Opposing to this, 532 nm mitigates the fluorescence termination partially, however, the spectral feature is broad and yields a lower fluorescence count rate. The difference between the two situations is discussed in the main text.

We repeat the long-term PLE measurements conducted in the main text on emitter 4 for three different power settings. The charge stabilisation is achieved by a continuously applied 445 nm laser with 70 µW of laser power. The resonant saturation power $P_{\mathrm{sat}}$ of the emitter is about 3 nW. All measurements are conducted over the course of about one hour. The low power scan in Supplementary Figure 11a) shows the stability of the emission line when a laser power of 0.1 nW, far below saturation, is applied. The single scan linewidth of emitter 4 is 43 MHz on average, which is slightly above the lifetime limited linewidth of 31 MHz. The summed linewidth of all scans amounts to 47.5 MHz. In b) 2.5 nW of resonant laser power are applied, which is close to the saturation power. The average linewidth of the slightly power broadened single line scans is 48 MHz, while the summed linewidth of all scans adds up to 50 MHz. In c) we explore the power regime significantly exceeding the saturation power at a resonant laser power of 20 nW. The average linewidth of a single line scan is about 121 MHz and the summed linewidth of all scans amounts to 124 MHz.

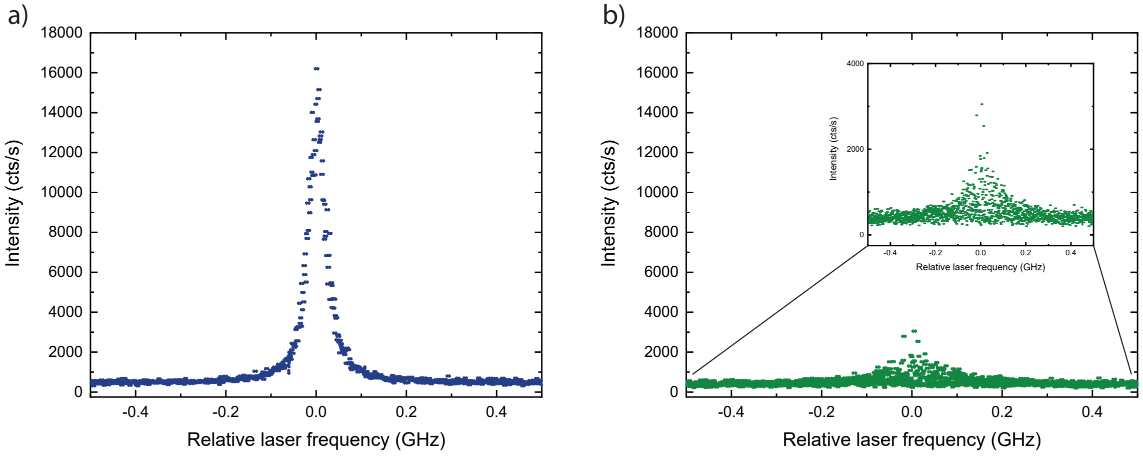


Supplementary Figure 10: **Comparison of blue and green charge stabilisation: a)** Application of 10 µW of 445 nW charge stabilisation radiation, while the laser scan across the C-transition is conducted with 1 nW of resonant laser power. A clear and narrow spectral feature is observed. **b)** Same measurement conducted with 10 µW of 532 nW charge stabilisation radiation. The spectral line is broadened significantly and the count rate on the resonance maximum is severely reduced compared to the blue charge stabilisation.

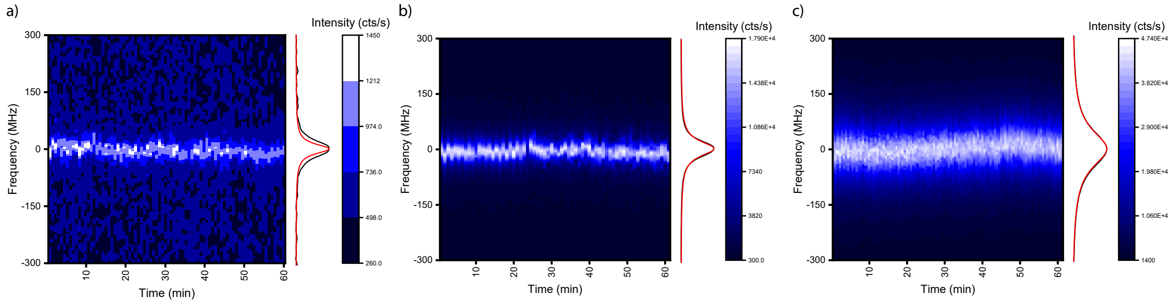


Supplementary Figure 11: **Long-term PLE measurements emitter 4:** A charge stabilisation laser power of 70 µW at 445 nm is applied. The resonance scan is conducted at **a)** 0.1 nW, which is about a factor of 30 below saturation power, **b)** 2.5 nW$\approx P_{\mathrm{sat}}$ and **c)** 20 nW$\gg P_{\mathrm{sat}}$. For all power settings, the resonance line stays very stable and the comparison of the sum of all scans for each measurement (black solid line) to the lifetime limited linewidth of 31 MHz in **a)** and the average single line scan in **b)** with a power broadened linewidth of 48 MHz and **c)** 121 MHz (red solid line) is plotted on the right of each graph.

# Supplementary note 7: Density matrix formalism

The simulations of the CPT experiments in the main paper employ a simple three level density matrix formalism. The three levels involved are the two spin ground states $|1\downarrow\rangle, |2\uparrow\rangle$ and the excited state $|A\downarrow\rangle$. The carrier (sideband) of our laser is addressing the SF (SC) transition A2 (A1) and the respective Rabi frequency is labeled $\Omega_{\mathrm{SF}}$ ($\Omega_{\mathrm{SC}}$) with the laser detuning from resonance being $\Delta_{\mathrm{SF}}$ ($\Delta_{\mathrm{SC}}$). The full Hamiltonian in rotating wave approximation is given by

$$H = \hbar \begin{pmatrix} 0 & 0 & \frac{\Omega_{\mathrm{SF}}}{2} \\ 0 & \Delta_{\mathrm{SF}} - \Delta_{\mathrm{SC}} & \frac{\Omega_{\mathrm{SC}}}{2} \\ \frac{\Omega_{\mathrm{SF}}}{2} & \frac{\Omega_{\mathrm{SC}}}{2} & \Delta_{\mathrm{SF}} \end{pmatrix}.$$

While the Hamiltonian and Schrödingers equation describe the coherent processes in a quantum system, we employ the master equation

$$\dot{\rho}(t) = -\frac{i}{\hbar}[\mathcal{H}, \rho] + \mathcal{L} + \mathcal{D}$$

to extent the model to cover also incoherent processes. The spontaneous decay from the excited state $|\mathrm{A}\downarrow\rangle$ into the ground states or the thermalisation between the ground states is implemented utilising the Lindblad operators

$$\mathcal{L}_{ij} = C_{ij}\rho C_{ij}^{\dagger} - \frac{1}{2}(C_{ij}^{\dagger}C_{ij}\rho^{\dagger} + \rho C_{ij}^{\dagger}C_{ij}),$$

describing the decay from state $|i\rangle$ into the state $|j\rangle$. We here introduced the collapse operators

$$C_{ij} = \sqrt{\gamma_{ij}}\,|i\rangle\,\langle j|\,,$$

with the decay rate $\gamma_{ij}$. The Lindblad superoperator is now the sum over all decay paths possible within the system and thus given by

$$\mathcal{L} = \sum_{\substack{i,j\\ i\neq j}} \mathcal{L}_{ij}.$$

These decays occur on the SF and SC transitions with rates $\gamma_{\mathrm{SF/SC}}$ , as well as for the spin population thermalisation between the ground states $|1\downarrow\rangle$ and $|2\uparrow\rangle$ via the rates $\gamma_{21/12}$ which are defined by the common rate $\gamma_{\mathrm{spin}}$, that is measured in the $T_1$ measurements, by the formula

$$\gamma_{21/12} = \frac{\gamma_{\mathrm{spin}}}{2}\cdot\alpha_{\mathrm{therm}}\cdot\exp(\pm\frac{\hbar\Delta_{\uparrow\downarrow}}{2k_{\mathrm{B}}T}),$$

with

$$\alpha_{\mathrm{therm}} = \frac{1}{\exp(\frac{\hbar\Delta_{\uparrow\downarrow}}{2k_{\mathrm{B}}T}) + \exp(-\frac{\hbar\Delta_{\uparrow\downarrow}}{2k_{\mathrm{B}}T})}.$$

This rate is evaluated at a temperature $T$=1.7 K and a magnetic field of $B$=200 mT that leads to a Zeeman splitting of $\Delta_{\uparrow\downarrow}$=3.878 GHz between the spin ground states. We furthermore model the decoherence between the ground states as a pure dephasing of state $|2\uparrow\rangle$ with a rate $\gamma_{22}$ as

$$\mathcal{D} = \gamma_{22}(\rho_{22}\,|2\rangle\,\langle 2| - \frac{1}{2}\{|2\rangle\,\langle 2|\,\rho + \rho\,|2\rangle\,\langle 2|\})$$

from which one can directly derive a spin dephasing time $T_2^* = \frac{1}{\pi\gamma_{22}}$. The mathematical concept derived so far is sufficient to govern the full evolution of the density matrix and thereby the quantum system. However, for computational purposes it is more convenient using the Liouville super operator $\mathscr{L}$, which satisfies

$$\dot{\vec{\rho}} = \mathscr{L}\vec{\rho}. \tag{1}$$

Please note, that the density 3x3 matrix is now rewritten as a 9 dimensional vector, which is indicated by the vector label of $\vec{\rho}$. The matrix entries have been rearranged in the following way:

$$\begin{pmatrix} \rho_{11} & \rho_{12} & \rho_{13}\\ \rho_{21} & \rho_{22} & \rho_{23}\\ \rho_{31} & \rho_{32} & \rho_{33} \end{pmatrix} \longrightarrow \begin{pmatrix} \rho_{11}\\ \rho_{12}\\ \vdots\\ \rho_{32}\\ \rho_{33} \end{pmatrix}.$$

For the explicit expression of the operator $\mathscr{L}$, it is useful to define an effective Hamiltonian $\mathcal{H}_{\mathrm{eff}}$ as

$$\mathcal{H}_{\mathrm{eff}} = \mathcal{H} - \frac{i\hbar}{2}\left(\sum C_{ij}^{\dagger}C_{ij} + \mathcal{D}^{\dagger}\mathcal{D}\right).$$

Utilising the effective Hamiltonian we can calculate $\mathscr{L}$ according to [4] as

$$\mathscr{L} = i(\mathbb{1}_3\otimes\mathcal{H}_{\mathrm{eff}}^{\dagger} - \mathcal{H}_{\mathrm{eff}}\otimes\mathbb{1}_3) + \sum_{\substack{i,j\\ i\neq j}} C_{ij}\otimes C_{ij}^{\dagger} + \mathcal{D}\otimes\mathcal{D}^{\dagger}.$$

| $\Delta^{\mathrm{m}}_{\uparrow\downarrow}$ (GHz) | $T^{\mathrm{m}}$ (K) | $\gamma^{\mathrm{m}}_{\mathrm{spin}}$ (GHz) | $\gamma^{\mathrm{m}}_{12}$ (GHz) | $\gamma^{\mathrm{m}}_{21}$ (GHz) | $\gamma^{\mathrm{m}}_{\mathrm{SC}}$ (GHz) | $\gamma_{\mathrm{SF}}$ (GHz) | $\gamma_{22}$ (GHz) |
|---|---|---|---|---|---|---|---|
| 3.878 | 1.7 | $\frac{1}{2\pi\cdot 22000000}$ | $\frac{\gamma_{\mathrm{spin}}}{2}\cdot\alpha_{\mathrm{therm}}\cdot\exp(-\frac{\hbar\Delta_{\uparrow\downarrow}}{2k_{\mathrm{B}}T})$ | $\frac{\gamma_{\mathrm{spin}}}{2}\cdot\alpha_{\mathrm{therm}}\cdot\exp(\frac{\hbar\Delta_{\uparrow\downarrow}}{2k_{\mathrm{B}}T})$ | $\frac{1}{2\pi\cdot 7}$ | $\frac{1}{2\pi\cdot 7}\cdot\frac{1}{650}$ | $\frac{1}{\pi\cdot 5000}$ |

Supplementary Table 1: **Simulation Parameters:** Listed are the parameters that were used in or extracted from the power dependent CPT simulations.

The advantage of this representation is that the solution of equation 1 can be calculated in a straightforward manner as

$$\vec{\rho} = \exp(2\pi\mathscr{L}t)\vec{\rho}_0,$$

where $\vec{\rho}_0$ describes the initial state of the quantum system. It is important to note, that this solution is only valid for the operator $\mathscr{L}$ being time invariant. The computational overhead of this formalism is strongly reduced compared to solving the nine coupled differential equations resulting from the master equation. For the CPT experiments we have to be sure to be in the steady state thus we choose the evaluation time $t$ =1 s in the experiment. The spectral scanning of the sideband over the SC transition in the experiment is simulated by varying the detuning $\Delta_{\mathrm{SC}}$.

The parameters that we either extract from the simulations or that are measured independently (measured values are indicated by a superscript "m") are listed in Supplementary Table 1. All frequency values are in units of GHz. The Rabi frequencies are power dependent and therefore not occuring in the table but rather being specified for each simulation independently.

In Supplementary Figure 12 we present the power dependent CPT measurements, which we use to pinpoint the exact numbers for $\gamma_{22}$, the ratio $\eta$ between the decay rate of the allowed SC transition and the spin forbidden SF transition and the Rabi frequencies. We further confirm the value of $\eta = 650(100)$ by pumping the spin from $|1\downarrow\rangle$ to $|2\uparrow\rangle$ for two different laser powers and fitting the measurements with our model. The laser power ratio $r_{\mathrm{power}}$ between the power being applied to the SF transition via the carrier of the EOM and the power applied to the SC transition generated in the first sideband of the EOM can be directly calculated from the formula

$$r_{\mathrm{power}} = \frac{P_{\mathrm{SF}}}{P_{\mathrm{SC}}} = \left(\frac{\Omega_{\mathrm{SF}}}{\Omega_{\mathrm{SC}}}\right)^2 \eta.$$

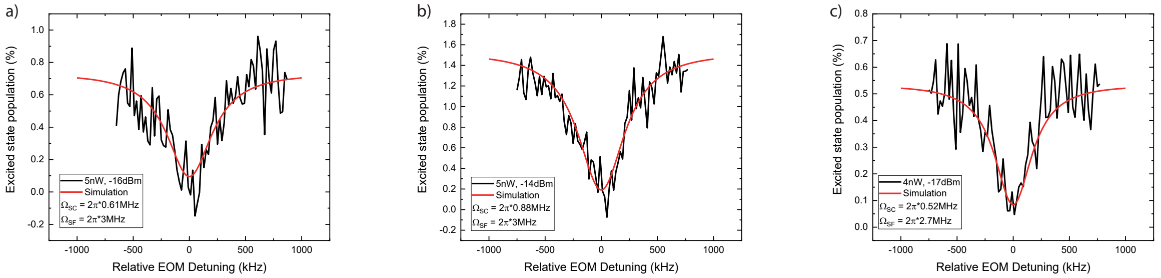


Supplementary Figure 12: **CPT measurements on emitter 2:** The measurements are conducted for different laser powers and different strength of the EOM sideband which is indicated by the different microwave power in dbm. The extracted Rabi frequencies and the ratio between the laser intensities for the different powers are **a)** $\Omega_{\mathrm{SC}} = 2\pi\cdot 0.61$MHz, $\Omega_{\mathrm{SF}} = 2\pi\cdot 3$MHz, $r_{\mathrm{power}} \approx 15700$, **b)** $\Omega_{\mathrm{SC}} = 2\pi\cdot 0.88$MHz, $\Omega_{\mathrm{SF}} = 2\pi\cdot 3$MHz, $r_{\mathrm{power}} \approx 7500$, **c)** $\Omega_{\mathrm{SC}} = 2\pi\cdot 0.52$MHz, $\Omega_{\mathrm{SF}} = 2\pi\cdot 2.7$MHz, $r_{\mathrm{power}} \approx 17500$. We furthermore extract the parameter $\eta = 650$ and the spin dephasing time $T_2^* = 5000$ns when fitting these measurements and the lowest power measurement in the main text.

# References

[1] Gali, A. & Maze, J. R. Ab initio study of the split silicon-vacancy defect in diamond: Electronic structure and related properties. *Phys. Rev. B* **88**, 235205 (2013). URL `https://link.aps.org/doi/10.1103/PhysRevB.88.235205`.

[2] Görlitz, J. *et al.* Spectroscopic investigations of negatively charged tin-vacancy centres in diamond. *New Journal of Physics* **22**, 013048 (2020). URL `https://doi.org/10.1088/1367-2630/ab6631`.

[3] Thiering, G. & Gali, A. Ab initio magneto-optical spectrum of group-IV vacancy color centers in diamond. *Phys. Rev. X* **8**, 021063 (2018). URL `https://link.aps.org/doi/10.1103/PhysRevX.8.021063`.

[4] Am-Shallem, M., Levy, A., Schaefer, I. & Kosloff, R. Three approaches for representing lindblad dynamics by a matrix-vector notation. *arxiv* (2015). `1510.08634`.
